# Supplementary material for: A Survey on Point-of-Interest Recommendation: Models, Architectures, and Security
Source: arXiv:2410.02191 source file (2025-03-10)
Supplement: Supplementary file 1 [file appendix.tex]

\section*{ADDITIONAL EXPERIMENTS} \label{app}

\noindent \textbf{Evaluation Platform.}
%The implementation of \texttt{BEPN4DE} is based on 
All the methods are implemented in Python 3.6. and PyTorch 1.7.0. The experiments are conducted on a server with 10-cores of Intel(R) Core(TM) i9-9820X CPU @ 3.30GHz 64.0GB RAM and one Nvidia GeForce RTX 2080 GPU. The datasets and codes are at the anonymous link~\footnote{\url{https://www.dropbox.com/sh/7ktjq6h3zi99wlp/AABGXzV1GnQq2JKzaYmjjkQ6a?dl=0}}. %to reproduce the results.

\noindent \textbf{(1) Effectiveness when varying $\alpha$ for the multi-task objective.} 
$\alpha$ controls the importance between the main task of detour extraction and the auxiliary task of abnormal detection on road segments in our multi-task loss function.
We vary $\alpha$ from 0.0 to 0.4 to study the effectiveness. 
Table~\ref{tab:alpha} reports the performance in terms of F1-score. 
When $\alpha$ is set to 0.0, our models reduce to the vanilla Pointer Network with only the main task of detour extraction, and the performance drops by around 9\%. It illustrates the power of the multi-task learning that uses an auxiliary task to enhance the performance of detour extraction. 
Further, observe that the F1 score increases and then decreases when $\alpha$ increases, and reaches the peak when $\alpha = 0.2$. Therefore, we use $\alpha=0.2$ by default, since it provides the best accuracy of detour extraction.

\noindent \textbf{(2) Effectiveness when varying $\delta$ in Travel Frequency Feature.}
Parameter $\delta$ is a threshold to generate binary travel frequency feature vector of a given trajectory in Section \ref{sec:encoder}.
Intuitively, $\delta$ controls the effects of modeling whether road segments are in a detour or not.
We vary $\delta$ from 0.3 to 0.7 and report the F1 scores of our methods  \texttt{BEPN4DE} and \texttt{BEPN4DE+} in  Table~\ref{tab:delta}. The performance increases and then drops when $\delta$ increases, and reaches the peak at $\delta=0.4$.
The intuition is that a small $\delta$ falsely models  anomalous road segments as normal (i.e., set to 1 in the binary travel frequency vector), which causes many detour-related road segments ignored in the feature vector, and vice versa. Therefore, a too small/large $\delta$ will lead to degraded performance. We set $\delta=0.4$ by default,  as it achieves the best $F_1$ score.

% the effects of simplification $\lambda$ (i.e., the parameter controlled the step of uniformly dropping points from a trajectory) for \texttt{BEPN4DE+}. As expected, we observe the $F_1$-score
% decreases with  $\lambda$ increases. This is because with a larger $\lambda$, the model tends to drop more points, which leads the information captured from the trajectory to become fewer and incomplete, but its efficiency improves with more points  dropped. 

\begin{table}[ht]
\setlength{\tabcolsep}{10pt}
\centering
\caption{F1 results when varying $\alpha$ for \texttt{BEPN4DE} and \texttt{BEPN4DE+}.}
%\vspace*{-3mm}
%\small
\begin{tabular}{|c|c|c|c|c|c|c|}
\hline
Parameter & $\alpha=0.0$ & $\alpha=0.1$ & $\alpha=0.2$ & $\alpha=0.3$ & $\alpha=0.4$ \\ \hline
\texttt{BEPN4DE} &0.802 &0.820 &\textbf{0.864} &0.855 &0.829 \\ \hline
\texttt{BEPN4DE+}&0.795 &0.818 &\textbf{0.851} &0.833 &0.809 \\ \hline
\end{tabular}
\label{tab:alpha}
%\vspace*{-2mm}
\end{table}

\begin{table}[ht]
\setlength{\tabcolsep}{10pt}
\centering
\caption{F1 results when varying $\delta$ for \texttt{BEPN4DE} and \texttt{BEPN4DE+}.}
%\vspace*{-3mm}
%\small
\begin{tabular}{|c|c|c|c|c|c|c|}
\hline
Parameter & $\delta=0.3$ & $\delta=0.4$ & $\delta=0.5$ & $\delta=0.6$ & $\delta=0.7$ \\ \hline
\texttt{BEPN4DE} & 0.859 &\textbf{0.864} &0.844 &0.829 &0.827 \\ \hline
\texttt{BEPN4DE+} &0.841 &\textbf{0.851} &0.826 &0.810 &0.809 \\ \hline
\end{tabular}
\label{tab:delta}
%\vspace*{-2mm}
\end{table}

\begin{table}[ht]
\setlength{\tabcolsep}{10pt}
\centering
%\small
\caption{F1 results when varying $\rho$.}
%\vspace*{-2mm}
\begin{tabular}{|c|c|c|c|c|c|c|}
\hline
Parameter & $\rho=0.3$ & $\rho=0.4$ & $\rho=0.5$ & $\rho=0.6$ & $\rho=0.7$ \\ \hline
\texttt{BEPN4DE} &0.814 &\textbf{0.864} &0.858 &0.853 &0.862 \\ \hline
\texttt{BEPN4DE+}&0.803 &\textbf{0.851} &0.844 &0.838 &0.848 \\ \hline
\end{tabular}
\label{tab:rho}
%\vspace*{-2mm}
\end{table}

\begin{table}[]
\setlength{\tabcolsep}{12pt}
\centering
\caption{F1 results when varying $d$.}
%\vspace*{-3mm}
%\small
\begin{tabular}{|c|c|c|c|c|c|c|}
\hline
Parameter & $d=2$ & $d=2.5$ & $d=3$ & $d=3.5$ & $d=4$ \\ \hline
\texttt{BEPN4DE} &0.857 &\textbf{0.864} &0.854 &0.848 &0.852 \\ \hline
\texttt{BEPN4DE+}&0.841 &\textbf{0.851} &0.836 &0.831 &0.834 \\ \hline
\end{tabular}
\label{tab:d}
%\vspace*{-2mm}
\end{table}

\noindent \textbf{(3) Effectiveness when varying $\rho$ and $d$ in synthetic detour injection.} We study the effects of parameters $\rho$ and $d$ for generating detours of the weakly supervised model training. Table~\ref{tab:rho} and Table~\ref{tab:d} report the $F_1$ scores of the two parameters respectively, for \texttt{BEPN4DE} and \texttt{BEPN4DE+} on the testing set of Chengdu. As either $\rho$ or $d$ increases in Tables \ref{tab:rho} and \ref{tab:d} respectively, the performance improves and then degrades. Therefore, we set $\rho=0.4$ and $d=2.5$ for training.

\if 0
\noindent \textbf{(4) Efficiency evaluation when varying comparisons in global pruning.}
To compare different strategies incorporated in global pruning for extracting detours in a database, we randomly sample trajectories and construct a database with 0.5 million data points. We demonstrate these strategies in terms of effectiveness and efficiency. In particular, we provide the strategy without any pruning (denoted as ``Native''); and a random strategy (denoted as ``random''), which is to randomly prune trajectories in the database; and the proposed strategy, which prunes with a learned classifier (denoted as ``learned'').
In Figure~\ref{fig:index}, we take the \texttt{BEPN4DE+} model for example, and vary the parameter of pruning ratio from 0.5 to 0.9. We report the running time and $F_1$-score in the database via mapping the routes to ground truth. As expected, we observe the effectiveness degrades as pruning more trajectories, because the detour trajectories would be filtered with a larger pruning ratio. Also, the learned strategy is much better than the random strategy and close to the Naive strategy (i.e., without pruning), since it can accurately prune the normal trajectories with a learned classifier for this task. In contrast, the random strategy performs the worst as it is to randomly drop some of the trajectories from the database, though it runs slightly fast. The results provided by \texttt{BEPN4DE} model show similar trends and thus omitted.

\begin{figure}
	%\hspace{-.8cm}
	\centering
	\begin{tabular}{c c}
		\begin{minipage}{3.7cm}
			\includegraphics[width=3.9cm]{figures/pruning_chengdu_f1.pdf}
		\end{minipage}
		&
		\begin{minipage}{3.7cm}
			\includegraphics[width=3.9cm]{figures/pruning_chengdu_time.pdf}
		\end{minipage}
		\\
		(a) $F_1$-score
		&
		(b) Time cost (s)
	\end{tabular}
	%\vspace{-3mm}
	\caption{Comparison with different strategies in global pruning.}\label{fig:index}
	%\vspace{-3mm}
\end{figure}
\fi
